# Supplementary material for: Potential energy surface prediction of Alumina polymorphs using graph neural network
Source: arXiv:2301.12059 source file (2023-01-28)
Supplement: Supplementary file 1 [file supplementary.tex]

\section{Supplementary}

\subsection{Prediction of energy at equilibrium}
\label{sec:equilibrium}
Xie \etal \cite{cgcnn} train their CGCNN model to predict formation energy per atom $\left(\Delta E_f\right)$ using a large number of equilibrium crystal structures obtained from the Materials Project \cite{materials_project}. Since $\left(\Delta E_f\right)$ for a large number of crystals can span across a wide range (approximately 8.5 eV/atom), such a model will not be able to accurately predict the small energy differences across different polymorphs of the same composition. However, in this work we train our CGCNN based models to predict the PES of various polymorphs of alumina through training on distorted input structures obtained from MD simulations. Due to this training data, we expect our model that has the same architecture as Xie et.al to perform better in predicting the energy differences of the alumina polymorphs. The mean absolute errors of predictions from the two approaches is shown in table \ref{tab:equilibrium}. As expected, our model  significantly outperforms the previous CGCNN model suggesting that the CGCNN architecture is transferable to predict small energy changes typically seen in distortions just by modifying the training data without any modifications to the neural network architecture. In the next upcoming subsections, we will discuss the PES predictions of alumina for various supercell sizes, temperature and polymorphs.

\begin{table}[]
	\centering
	\begin{tabular}{lC{6em}C{6em}}
		\hline
		%					& \multicolumn{2}{c}{MAE/atom}	\\
		%		\cline{2-3}
		Phase		& Xie \etal	& Our work			\\
		\hline
		Orthorhombic		& 0.0208	& 0.004				\\
		Trigonal	& 0.0466	& 0.0052			\\
		Cubic 		& 0.0152	& 0.0017			\\
		\hline
	\end{tabular}
	\caption{\label{tab:equilibrium} Mean Absolute Error per atom (MAE/atom) of CGCNN model on test dataset of different polymorphs using models trained on setups as defined in Sec. \ref{sec:equilibrium}.}
\end{table}

\subsection{Transferable CGCNN models across different Polymorphs}
\label{sec:transfer_poly}
One of the major challenges in materials and chemistry arises from the difficulty in transfering information, model and knowledge across different crystal structures. A model that can learn properties such as potential energy, from equilibrium and distorted configurations of some crystal structures and predict for new crystal structures with minimal data would be a very useful tool in accelerating materials discovery. As a preliminary step toward this goal, in this work, we study the transferability of CGCNN models across different polymorphs of alumina. We consider four phases of alumina - orthorhombic (Pbca and Pna2$_{1}$), trigonal, and cubic. For the first set of experiments, we predict the potential energy of the different polymorphs based on the training data from another polymorph (\textit{aka} zero shot learning). Similar to temperature study, here we use all the data pertaining to a polymorph (10,000 configurations) to train the model. The results are shown in Table \ref{tab:al_poly_exp1}. 

{\color{red} [Explanations]} {\color{red} As observed from the data, the model trained on crystal structures with lower symmetry (orthorhombic) is able to better predict the potential energy of crystal structures with higher symmetry (cubic), but not the other way around (see Fig. \ref{fig:bond_dist}, \ref{fig:dos}).}

\begin{figure}[h!]
	\includegraphics[width = 0.7\linewidth]{./figures/dos.eps}
	\caption{\label{fig:dos} Density of energy distribution of Alumina polymorphs}
\end{figure}

In order to understand how the model accuracy improves when trained with heterogeneous data, we train the model with data from multiple polymorphs to predict potential energy of orthorhombic (Pbca) polymorph. We choose orthorhombic (Pbca) for our analysis because the error in PES prediction was the highest as shown in Table \ref{tab:al_poly_exp1}. The results for this analysis is shown in Table \ref{tab:al_poly_exp2}. We observe that if we restrict the training data to a total of 9,900 configurations (each polymorph has 3,300 data points), the error in prediction is about 0.4294 meV/atom suggesting that training on diverse dataset can improve the transferability of the model. However, if we incorporate all the data from the three polymorphs (30,000 configurations in total), the model error reduces to 0.035eV/atom suggesting that the transferability of the model can be improved by increasing both the volume and variety of training data.

\begin{table}[]
  	\centering
  	\begin{tabular}{lcccc}
	    \hline
	    Phase & Orthorhombic (Pbca)  & Trigonal & Cubic  & Orthorhombic (Pna2$_{1}$) \\
	    \hline
		Orthorhombic (Pbca)    & 0.0008 & 0.0405   & 0.0493 & 0.0289 \\
		Trigonal & 1.1159 & 0.0009   & 0.045  & 0.2638 \\
		Cubic    & 5.0642 & 0.0456   & 0.0007 & 0.3871 \\
		Orthorhombic (Pna2$_{1}$)   & 2.4496 & 0.6063   & 0.7392 & 0.0007 \\
	    \hline
	\end{tabular}
  	\caption{\label{tab:al_poly_exp1} MAE/atom of CGCNN model on test data of 240 atom alumina for three different polymorphs. The row phase denotes that the model was trained using the data for that particular polymorph and column phase indicates that the trained model was used to predict the potential energy for that polymorph. Refer to Sec. \ref{sec:transfer_poly} for more details.}
\end{table}

\begin{table}[]
  	\centering
  	\begin{tabular}{lc}
	   	\hline
	    Mixture & MAE/atom \\
	    \hline
		Cubic + Trigonal + Orthorhombic (Pna2$_{1}$)(3300 each) 	& 0.4294          \\
	    Cubic + Trigonal + Orthorhombic (Pna2$_{1}$)    			& 0.035           \\
	    \hline
	\end{tabular}
  	\caption{\label{tab:al_poly_exp2} MAE/atom of CGCNN model on test data of 240 atom alumina othorhombic (Pbca) polymorph using a mixture of data for different alumina polymorphs in training data. Please refer to Sec. \ref{sec:transfer_poly} for details.}
\end{table}
